# Supplementary material for: Asymptotic calibration of projected residual processes in multilevel linear mixed models
Source: arXiv:2611.40802 source file (2026-11-30)
Supplement: Supplementary file 1 [file labels-supplement.tex]

\makeatletter
\global\@namedef{r@S-tab:statement-map}{{S1}{2}{Results of the paper, the supplement statements that prove them, and the Lean modules that formalise them. Section~\ref {sec:si-lean} states the form of the Lean theorems for each statement. The file \texttt {lean/PROOF\_MAP.md} lists the Lean theorems by manuscript label}{table.1}{supplement.pdf}}
\global\@namedef{r@S-sec:setting}{{S1}{3}{Setting and notation}{section.1}{supplement.pdf}}
\global\@namedef{r@S-sec:si-conditions}{{S1}{3}{Setting and notation}{section.1}{supplement.pdf}}
\global\@namedef{r@S-sec:model}{{S1.1}{3}{The model}{subsection.1.1}{supplement.pdf}}
\global\@namedef{r@S-eq:LMM_multi_level}{{S1}{3}{The model}{equation.1.1}{supplement.pdf}}
\global\@namedef{r@S-eq:Vn}{{S2}{3}{The model}{equation.1.2}{supplement.pdf}}
\global\@namedef{r@S-eq:P}{{S3}{3}{The model}{equation.1.3}{supplement.pdf}}
\global\@namedef{r@S-eq:HS}{{S4}{3}{The model}{equation.1.4}{supplement.pdf}}
\global\@namedef{r@S-eq:P-annihilates}{{S5}{3}{The model}{equation.1.5}{supplement.pdf}}
\global\@namedef{r@S-sec:processes}{{S1.2}{3}{The processes}{subsection.1.2}{supplement.pdf}}
\global\@namedef{r@S-eq:sigma-lambda}{{S6}{3}{The processes}{equation.1.6}{supplement.pdf}}
\global\@namedef{r@S-eq:oracleOS}{{S7}{4}{The processes}{equation.1.7}{supplement.pdf}}
\global\@namedef{r@S-eq:oracle-process}{{S8}{4}{The processes}{equation.1.8}{supplement.pdf}}
\global\@namedef{r@S-eq:kernel}{{S9}{4}{The processes}{equation.1.9}{supplement.pdf}}
\global\@namedef{r@S-eq:estimated-quantities}{{S10}{4}{The processes}{equation.1.10}{supplement.pdf}}
\global\@namedef{r@S-eq:primary-process}{{S11}{4}{The processes}{equation.1.11}{supplement.pdf}}
\global\@namedef{r@S-eq:secondary-process}{{S12}{4}{The processes}{equation.1.12}{supplement.pdf}}
\global\@namedef{r@S-eq:fitted-quantities}{{S13}{4}{The processes}{equation.1.13}{supplement.pdf}}
\global\@namedef{r@S-sec:tests}{{S1.3}{5}{Test statistics and $p$-values}{subsection.1.3}{supplement.pdf}}
\global\@namedef{r@S-eq:test-statistics}{{S14}{5}{Test statistics and $p$-values}{equation.1.14}{supplement.pdf}}
\global\@namedef{r@S-eq:p-value}{{S15}{5}{Test statistics and $p$-values}{equation.1.15}{supplement.pdf}}
\global\@namedef{r@S-eq:mc-p-value}{{S16}{5}{Test statistics and $p$-values}{equation.1.16}{supplement.pdf}}
\global\@namedef{r@S-sec:si-proofs}{{S2}{5}{Proofs for the sections on the tests and their validity}{section.2}{supplement.pdf}}
\global\@namedef{r@S-sec:minp-scales}{{S2.1}{6}{Finite-sample and asymptotic calibration of the minimum-$p$ rule}{subsection.2.1}{supplement.pdf}}
\global\@namedef{r@S-sec:si-rank}{{S2.1}{6}{Finite-sample and asymptotic calibration of the minimum-$p$ rule}{subsection.2.1}{supplement.pdf}}
\global\@namedef{r@S-prop:joint-statistic-ranks}{{S1}{6}{Joint calibration of a finite set of statistics}{theorem.1}{supplement.pdf}}
\global\@namedef{r@S-sec:rank-kernel}{{S2.1}{7}{Finite-sample and asymptotic calibration of the minimum-$p$ rule}{Item.3}{supplement.pdf}}
\global\@namedef{r@S-sec:oracle}{{S2.2}{7}{Exact orthogonality and the universal modulus}{subsection.2.2}{supplement.pdf}}
\global\@namedef{r@S-lem:orthogonality}{{S2}{7}{Exact orthogonality}{theorem.2}{supplement.pdf}}
\global\@namedef{r@S-eq:oracle-product-law}{{S17}{7}{Exact orthogonality and the universal modulus}{equation.2.17}{supplement.pdf}}
\global\@namedef{r@S-lem:modulus}{{S3}{7}{Universal covariance modulus}{theorem.3}{supplement.pdf}}
\global\@namedef{r@S-eq:universal-modulus}{{S18}{7}{Universal covariance modulus}{equation.2.18}{supplement.pdf}}
\global\@namedef{r@S-eq:universal-modulus-secondary}{{S19}{7}{Universal covariance modulus}{equation.2.19}{supplement.pdf}}
\global\@namedef{r@S-sec:si-exact}{{S2.3}{8}{Gaussian draws and rotations}{subsection.2.3}{supplement.pdf}}
\global\@namedef{r@S-lem:residual-space}{{S4}{8}{Residual-space identities and the conditional law of the projected residual}{theorem.4}{supplement.pdf}}
\global\@namedef{r@S-eq:likelihood-split}{{S20}{8}{Residual-space identities and the conditional law of the projected residual}{equation.2.20}{supplement.pdf}}
\global\@namedef{r@S-lem:projected-anticoncentration}{{S5}{9}{Continuity uniform over nondegenerate projected grids}{theorem.5}{supplement.pdf}}
\global\@namedef{r@S-lem:radial-conditioning}{{S6}{10}{Radial conditioning}{theorem.6}{supplement.pdf}}
\global\@namedef{r@S-prop:gaussian-O}{{S7}{11}{Gaussian draws for the projected processes}{theorem.7}{supplement.pdf}}
\global\@namedef{r@S-eq:gaussian-O-conditions}{{S21}{12}{Gaussian draws for the projected processes}{equation.2.21}{supplement.pdf}}
\global\@namedef{r@S-sec:si-fixed-path}{{S3}{13}{Fixed-prediction limits, fitted weights and unit multipliers}{section.3}{supplement.pdf}}
\global\@namedef{r@S-sec:si-indicator-order}{{S3.1}{14}{Indicators with a fitted multivariable ordering}{subsection.3.1}{supplement.pdf}}
\global\@namedef{r@S-sec:shared-conditions}{{S4}{17}{Gaussian approximation with estimated orderings and scales}{section.4}{supplement.pdf}}
\global\@namedef{r@S-sec:oracle-conditions}{{S4.1}{17}{Conditions on the oracle process}{subsection.4.1}{supplement.pdf}}
\global\@namedef{r@S-eq:rho0}{{S22}{18}{Conditions on the oracle process}{equation.4.22}{supplement.pdf}}
\global\@namedef{r@S-eq:rho0-local}{{S23}{18}{Conditions on the oracle process}{equation.4.23}{supplement.pdf}}
\global\@namedef{r@S-prop:O3-sufficient}{{S8}{18}{Sufficient conditions for (O3) and (O3-L)}{theorem.8}{supplement.pdf}}
\global\@namedef{r@S-eq:random-limit-dominator}{{S24}{18}{Sufficient conditions for (O3) and (O3-L)}{equation.4.24}{supplement.pdf}}
\global\@namedef{r@S-sec:estimated}{{S4.2}{19}{Conditions on the estimated parameters}{subsection.4.2}{supplement.pdf}}
\global\@namedef{r@S-eq:plugin-remainders}{{S25}{19}{Conditions on the estimated parameters}{equation.4.25}{supplement.pdf}}
\global\@namedef{r@S-eq:feasible-identity}{{S26}{19}{Conditions on the estimated parameters}{equation.4.26}{supplement.pdf}}
\global\@namedef{r@S-sec:secondary}{{S4.3}{20}{Conditions on the secondary processes}{subsection.4.3}{supplement.pdf}}
\global\@namedef{r@S-eq:shared-fitted-quantities}{{S27}{20}{Conditions on the secondary processes}{equation.4.27}{supplement.pdf}}
\global\@namedef{r@S-eq:shared-modulus-secondary}{{S28}{20}{Conditions on the secondary processes}{equation.4.28}{supplement.pdf}}
\global\@namedef{r@S-eq:secondary-linearity}{{S29}{20}{Conditions on the secondary processes}{equation.4.29}{supplement.pdf}}
\global\@namedef{r@S-sec:results}{{S5}{21}{Oracle, primary and secondary Gaussian limits}{section.5}{supplement.pdf}}
\global\@namedef{r@S-sec:si-asymptotic}{{S5}{21}{Oracle, primary and secondary Gaussian limits}{section.5}{supplement.pdf}}
\global\@namedef{r@S-sec:oracle-results}{{S5.1}{21}{Oracle processes}{subsection.5.1}{supplement.pdf}}
\global\@namedef{r@S-thm:oracle}{{S9}{21}{Oracle processes}{theorem.9}{supplement.pdf}}
\global\@namedef{r@S-eq:conditional-modulus}{{S30}{21}{Oracle processes}{equation.5.30}{supplement.pdf}}
\global\@namedef{r@S-eq:AEC}{{S31}{21}{Oracle processes}{equation.5.31}{supplement.pdf}}
\global\@namedef{r@S-cor:FO}{{S10}{22}{Group counts in the oracle limit}{theorem.10}{supplement.pdf}}
\global\@namedef{r@S-sec:estimated-results}{{S5.2}{22}{Primary processes and parameter estimation}{subsection.5.2}{supplement.pdf}}
\global\@namedef{r@S-thm:estimated}{{S11}{22}{Primary processes with estimated parameters}{theorem.11}{supplement.pdf}}
\global\@namedef{r@S-eq:primary-expansion}{{S32}{22}{Primary processes with estimated parameters}{equation.5.32}{supplement.pdf}}
\global\@namedef{r@S-sec:secondary-results}{{S5.3}{22}{Secondary processes}{subsection.5.3}{supplement.pdf}}
\global\@namedef{r@S-thm:secondary}{{S12}{22}{Secondary processes}{theorem.12}{supplement.pdf}}
\global\@namedef{r@S-eq:secondary-identity}{{S33}{23}{Secondary processes}{equation.5.33}{supplement.pdf}}
\global\@namedef{r@S-eq:three-terms}{{S34}{23}{Secondary processes}{equation.5.34}{supplement.pdf}}
\global\@namedef{r@S-sec:pvalues}{{S5.4}{23}{Test statistics and $p$-values}{subsection.5.4}{supplement.pdf}}
\global\@namedef{r@S-prop:pvalues}{{S13}{23}{Asymptotic validity of the $p$-values}{theorem.13}{supplement.pdf}}
\global\@namedef{r@S-sec:implemented-statistics}{{S5.5}{24}{Statistics on the fitted-value grid}{subsection.5.5}{supplement.pdf}}
\global\@namedef{r@S-eq:implemented-statistics}{{S35}{24}{Statistics on the fitted-value grid}{equation.5.35}{supplement.pdf}}
\global\@namedef{r@S-lem:sampled-ks}{{S14}{25}{Sampled supremum}{theorem.14}{supplement.pdf}}
\global\@namedef{r@S-prop:implemented-pvalues}{{S15}{25}{Calibration of the implemented statistics}{theorem.15}{supplement.pdf}}
\global\@namedef{r@S-eq:empirical-integration}{{S36}{25}{Calibration of the implemented statistics}{equation.5.36}{supplement.pdf}}
\global\@namedef{r@S-sec:shared-minp-scales}{{S5.6}{26}{The minimum-$p$ rule across scales}{subsection.5.6}{supplement.pdf}}
\global\@namedef{r@S-prop:minp-scales}{{S16}{26}{Joint calibration over scales}{theorem.16}{supplement.pdf}}
\global\@namedef{r@S-sec:ml-F}{{S5.7}{27}{Verification of the estimation conditions for the fixed-part process}{subsection.5.7}{supplement.pdf}}
\global\@namedef{r@S-prop:ml-F}{{S17}{27}{ML and REML with bounded group sizes: the fixed-part process}{theorem.17}{supplement.pdf}}
\global\@namedef{r@S-sec:si-detection}{{S6}{28}{Behaviour under alternatives}{section.6}{supplement.pdf}}
\global\@namedef{r@S-sec:alternatives}{{S6}{28}{Behaviour under alternatives}{section.6}{supplement.pdf}}
\global\@namedef{r@S-sec:alternative-conditions}{{S6.1}{28}{Alternatives, pseudo-true parameters and the mean function}{subsection.6.1}{supplement.pdf}}
\global\@namedef{r@S-eq:alternative-model}{{S37}{28}{Alternatives, pseudo-true parameters and the mean function}{equation.6.37}{supplement.pdf}}
\global\@namedef{r@S-eq:mean-function}{{S38}{28}{Alternatives, pseudo-true parameters and the mean function}{equation.6.38}{supplement.pdf}}
\global\@namedef{r@S-sec:si-mean}{{S6.2}{28}{Mean functions under Gaussian alternatives}{subsection.6.2}{supplement.pdf}}
\global\@namedef{r@S-prop:mean-function}{{S18}{28}{Mean functions under Gaussian alternatives}{theorem.18}{supplement.pdf}}
\global\@namedef{r@S-eq:mean-function-formula}{{S39}{29}{Mean functions under Gaussian alternatives}{equation.6.39}{supplement.pdf}}
\global\@namedef{r@S-sec:si-consistency}{{S6.3}{30}{Consistency}{subsection.6.3}{supplement.pdf}}
\global\@namedef{r@S-thm:power}{{S19}{31}{Consistency}{theorem.19}{supplement.pdf}}
\global\@namedef{r@S-eq:secondary-tail}{{S40}{31}{Consistency}{equation.6.40}{supplement.pdf}}
\global\@namedef{r@S-sec:power-multipliers}{{S6.3}{33}{Consistency}{equation.6.40}{supplement.pdf}}
\global\@namedef{r@S-app:lemmas}{{S7}{34}{Auxiliary lemmas}{section.7}{supplement.pdf}}
\global\@namedef{r@S-lem:dyadic-modulus}{{S20}{34}{A finite-pattern Gaussian modulus}{theorem.20}{supplement.pdf}}
\global\@namedef{r@S-eq:dyadic-modulus}{{S41}{34}{A finite-pattern Gaussian modulus}{equation.7.41}{supplement.pdf}}
\global\@namedef{r@S-lem:anchored-supremum}{{S21}{34}{Supremum of an anchored sub-Gaussian process}{theorem.21}{supplement.pdf}}
\global\@namedef{r@S-lem:implemented-indicator}{{S22}{34}{Exact indicator statistics with ties}{theorem.22}{supplement.pdf}}
\global\@namedef{r@S-lem:covering}{{S23}{35}{Quantile covering bound}{theorem.23}{supplement.pdf}}
\global\@namedef{r@S-lem:finite-gaussian-limit}{{S24}{35}{Finite Gaussian mixtures and covariance limits}{theorem.24}{supplement.pdf}}
\global\@namedef{r@S-lem:constructed-functional}{{S25}{35}{Tight limits from finite laws and equicontinuity}{theorem.25}{supplement.pdf}}
\global\@namedef{r@S-lem:localized-geometries}{{S26}{35}{Combining localized comparison geometries}{theorem.26}{supplement.pdf}}
\global\@namedef{r@S-lem:tight-finite-approximation}{{S27}{35}{Finite approximation of tight bounded paths}{theorem.27}{supplement.pdf}}
\global\@namedef{r@S-eq:finite-approximation}{{S42}{35}{Finite approximation of tight bounded paths}{equation.7.42}{supplement.pdf}}
\global\@namedef{r@S-lem:marked-supremum}{{S28}{36}{A uniform supremum bound for marked empirical processes}{theorem.28}{supplement.pdf}}
\global\@namedef{r@S-sec:si-simulations}{{S8}{36}{Simulation study and application: protocol and tables}{section.8}{supplement.pdf}}
\global\@namedef{r@S-sec:si-profile-sim}{{S8.1}{36}{Balanced design with skewed errors}{subsection.8.1}{supplement.pdf}}
\global\@namedef{r@S-sec:si-sim-protocol}{{S8.2}{36}{Designs and protocol}{subsection.8.2}{supplement.pdf}}
\global\@namedef{r@S-sec:si-sim-size}{{S8.3}{37}{Size}{subsection.8.3}{supplement.pdf}}
\global\@namedef{r@S-fig:sim-size}{{S1}{38}{Null rejection rates of the tests (CvM, minimum-$p$ rule, ML, Gaussian draws with $B=999$) against $n$ (log scale). Grey band: $0.05\pm 1.96$ Monte Carlo standard errors (5000 replicates; 2000 in the 10-item design, where $O_\varnothing $ has 5000). The five-centre and the 10-item designs keep the number of centres and of items fixed as $n$ grows. In the one-level design $O$ and $O_1$ coincide}{figure.1}{supplement.pdf}}
\global\@namedef{r@S-tab:sim-size}{{S2}{39}{Null rejection rates at $\alpha =0.05$ under ML, Gaussian draws ($B=999$ secondary processes, $R$ marks normalised by $\|\bm R\bm y\|/\sqrt r$), 5000 replicates per cell. Cells: every process ($O_\varnothing $, $O$ and the factor processes; in the one-level design $O_1=O$ is counted once), both statistics (KS, CvM), indicator weights, the five scales $c\in \{1,2,10,100,1000\}$ and the minimum-$p$ rule, that is, 14 cells per process. Min / Median / Max over these cells; Max $|z|$: largest standardised deviation $|\text {rate}-0.05|/\mathrm {SE}$ over these cells (Monte Carlo SE 0.003 at the nominal level; the cells share their data sets, so they are strongly dependent); $O_\varnothing $, $O$: CvM with the minimum-$p$ rule. Sing.: share of singular fits. In the five-centre design the number of centres stays 5 at every $n$}{table.2}{supplement.pdf}}
\global\@namedef{r@S-sec:si-sim-norm}{{S8.4}{39}{The normalisation of the projected marks}{subsection.8.4}{supplement.pdf}}
\global\@namedef{r@S-sec:si-sim-power}{{S8.5}{39}{Power, scales and the limits of Gaussian draws}{subsection.8.5}{supplement.pdf}}
\global\@namedef{r@S-tab:sim-size-maxdev}{{S3}{40}{Largest standardised deviation $\max |z|$, $z=(\text {rate}-0.05)/\mathrm {SE}$ with $\mathrm {SE}=\sqrt {0.05\cdot 0.95/m}$ for $m$ replicates, over the null cells of every process: first number over the CvM minimum-$p$ cells at every $n$ (one cell per $n$), second over all cells (KS and CvM, indicator weights, five scales and the minimum-$p$ rule, that is, 14 cells per $n$). Gaussian draws ($B=999$, $R$ marks normalised by $\|\bm R\bm y\|/\sqrt r$). Guide: the 95\% point of the maximum of $k$ independent $|N(0,1)|$ is 2.73 for $k=8$, 2.57 for $k=5$, 2.49 for $k=4$ (minimum-$p$ columns: $k$ = number of $n$) and 3.50, 3.38, 3.32 for $k=112, 70, 56$ (all cells); the cells of one design share their data sets and are positively dependent. ML: the replicates of Table~\ref {tab:sim-size-full} (5000, $n=250$ to 32\,000) and the crossed design with 10 items (2000, $n=250$ to 16\,000; $O_\varnothing $: 5000); REML: those of Table~\ref {tab:sim-size-reml} (1000, $n=250$ to 16\,000; 10 items 1000, 400 at $n=16000$). One level: $O_1=O$}{table.3}{supplement.pdf}}
\global\@namedef{r@S-fig:sim-power}{{S2}{40}{Rejection rates under four alternatives (CvM, minimum-$p$ rule, ML; 5000 replicates per point, 2000 to 3000 at $n\ge 8000$) against $n$ (log scale); thin line: 0.05. Slope 1 is the subject slope, slope 2 the centre slope (nested, three-level) or the item slope (crossed). $O_1$ orders by subjects, $O_2$ by centres or items, $O_3$ by items (three-level); $O_\varnothing $ was run under the alternatives that omit the quadratic term}{figure.2}{supplement.pdf}}
\global\@namedef{r@S-tab:sim-fixed-levels}{{S4}{41}{Designs in which $n$ grows while one grouping factor keeps a fixed number of groups: rejection rates at $\alpha =0.05$ (CvM, minimum-$p$ rule, ML, Gaussian draws with $B=999$, $R$ marks normalised by $\|\bm R\bm y\|/\sqrt r$). Top: nested design with 5 centres (random intercept) and $n/10$ subjects (random intercept and slope), 5000 replicates (SE 0.003 at 0.05), except under the alternatives at $n\ge 16000$ (2000 replicates, SE at most 0.011). Bottom: crossed design with 10 items (random intercept and slope on $x_2$) and $n/10$ subjects (random intercept and slope on $x_1$), every subject meets every item once; 2000 replicates (SE 0.005 at 0.05), except $O_\varnothing $ under $H_0$ (5000 replicates, SE 0.003) and the alternatives at $n=16000$ (400 replicates, SE 0.011). Omitted: the term left out of the fitted model. Sing.: share of singular fits (of the 2000 replicates in the 10-item design). --: no such process (level 2 omitted), or not run ($O_\varnothing $ under the alternatives that omit only a random term)}{table.4}{supplement.pdf}}
\global\@namedef{r@S-tab:sim-size-reml}{{S5}{42}{Null rejection rates at $\alpha =0.05$ under REML, Gaussian draws ($B=999$, $R$ marks normalised by $\|\bm R\bm y\|/\sqrt r$), 1000 replicates per cell; columns and cells as in Table~\ref {tab:sim-size} (SE 0.007 at the nominal level). The crossed design with 10 items has 1000 replicates at $n\le 4000$ and 400 at $n=16000$ (SE 0.011); Max $|z|$ uses the SE of each cell's replicates}{table.5}{supplement.pdf}}
\global\@namedef{r@S-fig:sim-benchmark}{{S3}{42}{Benchmark on the same 2000 replicates per cell (ML): rejection rates against $n$ (log scale) of the likelihood-ratio test of the omitted term (LRT), the RESET test and the tests of this paper (CvM, minimum-$p$ rule, Gaussian draws with $B=999$); thin line: 0.05. Slopes and processes as in Figure~\ref {fig:sim-power}}{figure.3}{supplement.pdf}}
\global\@namedef{r@S-tab:sim-power}{{S6}{43}{Rejection rates at $\alpha =0.05$ under the alternatives (CvM, minimum-$p$ rule over $c\in \{1,2,10,100,1000\}$; ML; Gaussian draws with $B=999$, $R$ marks normalised by $\|\bm R\bm y\|/\sqrt r$; 5000 replicates at $n\le 4000$, SE at most 0.007; at $n=16000$ 2000 replicates, SE at most 0.011). Factors: one level, subject; nested, subject $\subset $ centre; crossed, subject $\times $ item; five centres, subject $\subset $ centre; three-level, subject $\subset $ centre, $\times $ item. Omitted: the term left out of the fitted model (the data always contain both slopes). --: process not defined, or not run ($O_\varnothing $ was run under the alternatives that omit $x_1^2$; with only a slope omitted, its CvM rates on 2000 replicates are in Table~\ref {tab:sim-benchmark})}{table.6}{supplement.pdf}}
\global\@namedef{r@S-tab:sim-scales}{{S7}{45}{The minimum-$p$ rule against single smoothing scales at $n=4000$: rejection rates of the process aimed at the omitted term (CvM; ML; Gaussian draws with $B=999$, $R$ marks normalised by $\|\bm R\bm y\|/\sqrt r$; 5000 replicates, SE at most 0.007). Ind.: indicator weights; $c$: scale $\lambda =c/I$. Omitted: $x_1^2$, the slope of factor 1 or 2, both slopes, or a whole factor. Process: $O_\varnothing $ when $x_1^2$ is omitted, the process of the factor for one omitted slope, $O$ otherwise. Bold: best single scale; Adapt.: the data-driven rule of \citet {LMMpaper} (the statistics at the five scales standardised by their standard deviation over the $B+1$ processes, maximum over the scales, calibrated on the same secondary processes); $\Delta $: minimum-$p$ minus best single scale (the best scale is chosen after seeing the results, so $\Delta \le 0$ is expected)}{table.7}{supplement.pdf}}
\global\@namedef{r@S-sec:si-sim-oempty}{{S8.6}{45}{The process $O_\varnothing $}{subsection.8.6}{supplement.pdf}}
\global\@namedef{r@S-tab:sim-benchmark}{{S8}{46}{Benchmark on the same 2000 replicates per cell (ML): the targeted likelihood-ratio test of the omitted term ($\chi ^2_1$ for $x_1^2$; for an omitted slope, the boundary mixture $\tfrac 12\chi ^2_1+\tfrac 12\chi ^2_2$; under $H_0$ the LRT of $x_1^2$), the RESET test (squares and cubes of the centred fixed-part fitted values, $\chi ^2_2$), and the tests of this paper with CvM, indicator weights (Ind.) and the minimum-$p$ rule (Gaussian draws, $B=999$, $R$ marks normalised by $\|\bm R\bm y\|/\sqrt r$). SE at most 0.011}{table.8}{supplement.pdf}}
\global\@namedef{r@S-tab:sim-limits}{{S9}{47}{Limits of Gaussian draws. (a) Small samples with singular fits and few groups at the coarse factor (ML, Gaussian draws, $B=999$, $R$ marks normalised by $\|\bm R\bm y\|/\sqrt r$; 5000 replicates, the data sets of Table~\ref {tab:sim-size-full} at these $n$): null rejection rates of $O_\varnothing $ and $O$ (CvM, minimum-$p$ rule) among singular and nonsingular fits. Groups: numbers of groups per level. (b) Two constructed null cases with ML fits (2000 replicates, $B=999$, $O$ with $R$ marks normalised by $\|\bm R\bm y\|/\sqrt r$): Gaussian draws (G) against their rotations (E; Section~\ref {M-sec:exact-link}), on the same data and draws; in parentheses Gaussian draws with the primary marks divided by $\hat \sigma $ instead (the scale $\hat \sigma $ of \citealp {LMMpaper}); $\bar d$ is the mean radial factor $\|\bm R\bm y\|/(\hat \sigma \sqrt r)$, by which the two Gaussian versions differ. SE 0.005 at 0.05}{table.9}{supplement.pdf}}
\global\@namedef{r@S-tab:sim-oempty}{{S10}{47}{The process $O_\varnothing $ (projected marks $\bm R\bm y/\tilde \sigma $ ordered by $\bm X\widehat {\bm \beta }$; Gaussian draws, $B=999$; same replicates and secondary draws as the other processes). (a) Null rejection rates at $\alpha =0.05$, CvM, minimum-$p$ rule, by $n$; range: over the 14 cells of each row and $n$ (KS, CvM; indicator weights, five scales, minimum-$p$), out: cells outside the 99\% band $0.05\pm 2.576\,\mathrm {SE}$; replicates as in Tables~\ref {tab:sim-size-full} and \ref {tab:sim-size-reml} (10 items: 5000 under ML). (b) Rejection rates (CvM, minimum-$p$, ML) under the omitted $x_1^2$, $x_1^2$ and the subject slope, and the omitted interaction $x_1x_2$ (other data sets: the data contain $x_1x_2$ with coefficient 1; 5000 replicates, every process); max $O_l$: largest factor process; $\Delta $: $O_\varnothing $ minus $O$ on the same replicates with the Monte Carlo SE of the paired difference. Replicates of $O_\varnothing $ under $x_1^2$: 5000 at $n\le 4000$ (10 items: 2000), 2000 at $n=16000$ (10 items: 400)}{table.10}{supplement.pdf}}
\global\@namedef{r@S-sec:si-sim-nongauss}{{S8.8}{49}{Non-Gaussian errors and unequal error variances}{subsection.8.8}{supplement.pdf}}
\global\@namedef{r@S-sec:si-lexdec}{{S8.9}{49}{The lexical decision application: data, sensitivity and complete tables}{subsection.8.9}{supplement.pdf}}
\global\@namedef{r@S-tab:sim-nongauss}{{S11}{50}{Null rejection rates at $\alpha =0.05$ when the errors are not Gaussian or have unequal variances (null hypothesis: the fitted model is the data-generating model; CvM, minimum-$p$ rule; ML; Gaussian draws with $B=999$; projected marks normalised by $\|\bm R\bm y\|/\sqrt r$). Errors ($\sigma =1$): Gaussian; $t_5$: Student $t$ with 5 degrees of freedom divided by $\sqrt {5/3}$; $\chi ^2_4$: $(\chi ^2_4-4)/\sqrt 8$ (skewness 1.41, kurtosis 6); unequal variance: Gaussian with standard deviation $s_i=0.75+0.25\,(x_{1i}+x_{2i})$, linear in the fixed prediction $1+x_{1i}+x_{2i}$ (mean of $s_i^2$: 1.010). Gaussian random effects in every row. 2000 replicates per cell (Monte Carlo standard error 0.005 at 0.05; 99\% band 0.037 to 0.063); the Gaussian rows are replicates 1--2000 of the study with Gaussian errors. Sing.: singular fits. One level: $O_1=O$; --: no second factor. $^{\dagger }$1000 replicates (standard error 0.007; 99\% band 0.032 to 0.068), run where a projected process was above the band at $n=4000$ and higher than at $n=1000$}{table.11}{supplement.pdf}}
\global\@namedef{r@S-tab:app-lexdec}{{S12}{51}{Lexical decision data \citep [Section~7.1]{BaayenBook2008}: 1659 responses, 21 subjects crossed with 79 words. Fixed effects: accuracy, trial position, previous-item type by the word's mean weight rating, log frequency, native language by word length. Random effects: D1, word and subject intercepts; D2, also a by-subject trial slope; D3, also a length slope; slopes correlated with the subject intercept. I1--I3: the same models for $-1000/\mathrm {RT}$. $p$-values (KS/CvM) with indicator weights (Ind.) and the minimum-$p$ rule; Gaussian draws, $B=999$; Joint: minimum-$p$ over the four processes and their scales. $\ell $: ML log-likelihood; $r=\rank \bm R$; LRT: likelihood-ratio statistic against the model above ($p$ in the text, from $\tfrac 12\chi ^2_{k}+\tfrac 12\chi ^2_{k+1}$, $k=1$ for D2, I2 and $k=2$ for D3, I3). Coding, $\mathrm {df}_a$ and all scales: Section~\ref {sec:si-lexdec}}{table.12}{supplement.pdf}}
\global\@namedef{r@S-fig:app-lexdec-paths}{{S4}{51}{Lexical decision data: primary path (black) and 50 of the $B=999$ secondary paths (grey) with indicator weights, against the ordering value. (a) $O_{\rm subj}$ under the random-intercept model D1 (log RT); (b) $O_{\rm subj}$ under D3, with by-subject slopes of trial position and word length; (c) $O_{\rm word}$ under D3; (d) $O_{\rm word}$ under the same model for $-1000/\mathrm {RT}$ (I3). CvM $p$-values with Gaussian draws (indicator weights / minimum-$p$ rule) in the panel titles}{figure.4}{supplement.pdf}}
\global\@namedef{r@S-tab:app-lexdec-exact}{{S13}{52}{Lexical decision data, fits of Tables~\ref {tab:app-lexdec} and \ref {tab:app-lexdec-sensitivity} (ML): $p$-values of the projected processes with Gaussian draws (G) and with their rotations (E; Section~\ref {M-sec:exact-link}): secondary marks $\sqrt r\,\bm R\bm \xi _b/\|\bm R\bm \xi _b\|$ in place of $\bm R\bm \xi _b$, on the same draws $\bm \xi _b$ ($B=999$, \texttt {Random.seed!(1)}); CvM, minimum-$p$ rule. Joint: the minimum-$p$ rule over the four projected processes and the five scales. G is the entry of Table~\ref {tab:app-lexdec}}{table.13}{supplement.pdf}}
\global\@namedef{r@S-tab:app-lexdec-sensitivity}{{S14}{52}{Lexical decision data, log RT: sensitivity of the tests of Table~\ref {tab:app-lexdec}. REML fits of D1--D3 ($\ell $: REML criterion $\times (-\tfrac 12)$); D3 refitted (ML) without the 78 responses whose standardised conditional residual under D3 is at least 2 in absolute value (the model criticism of the source; 72 of them are slow responses), $n=1581$, $\mathrm {df}=1438$ for $O_{\mathrm {word}}$; D4 (ML), which adds to D3 a by-word random slope of native language correlated with the word intercept, $\mathrm {df}=1439$ for $O_{\mathrm {word}}$, LRT against D3 with $p$ from $\tfrac 12\chi ^2_{1}+\tfrac 12\chi ^2_2$: $0.117$. REML LRT $p$: $6.4\times 10^{-8}$ and $1.2\times 10^{-5}$. $\hat d=\|\bm R\bm y\|/(\hat \sigma \sqrt r)$ between 0.9997 and 1.0008. Other columns as in Table~\ref {tab:app-lexdec}}{table.14}{supplement.pdf}}
\global\@namedef{r@S-fig:app-lexdec-path-O0}{{S5}{53}{Lexical decision data, model D3 (log RT, ML): $O_\varnothing $ at $c=1$, the CvM scale its minimum-$p$ rule selects, against the fixed prediction $\bm X\widehat {\bm \beta }$. Primary path in black; grey band: pointwise 2.5\% and 97.5\% quantiles of the $B=999$ secondary paths. CvM $p$-values (this scale / minimum-$p$ rule) in the title}{figure.5}{supplement.pdf}}
\global\@namedef{r@S-sec:si-sim-gaps}{{S8.10}{54}{What the study does not cover}{subsection.8.10}{supplement.pdf}}
\global\@namedef{r@S-sec:si-lean}{{S9}{54}{Formal verification}{section.9}{supplement.pdf}}
\makeatother
